# Supplementary material for: Wetting transition of active Brownian particles on a thin membrane
Source: arXiv:2111.02492 ancillary file (2021-11-03)
Supplement: Supplementary file 1 [file supp.pdf]

# Supplementary Material
# Wetting transition of active Brownian particles on a thin membrane

Francesco Turci* and Nigel B. Wilding
*H.H. Wills Physics Laboratory, Tyndall Avenue, Bristol, BS8 1TL, UK*

This supplementary material provides technical detail to complement the main text. It is arranged as follows. (S1): details of our model and simulation procedure; (S2): Definition of the asymmetry order parameter that characterises the wetting transition; (S3) Phenomenology of wetting in systems with fixed particle number and volume; (S4): Method for determining the distribution of sizes of bubbles in the high density phase; (S5): Definition of the local compressibility profile, its main features and aspects relevant to the discussion in the main text; (S6): Some details on the dynamics of events in which the liquid layer detaches from the barrier.

## S1. MODEL

Models of active Brownian particles (ABPs) have been extensively studied in the past in both two dimensions (2d) and (less often) in three dimensions (3d). We adopt the model proposed by Stenhammar et al. of repulsive active Brownian particles [1]. Here the particles interact exclusively via a repulsive, short-ranged interaction provided by the truncated and shifted Weeks-Chandler-Anderson potential

$$U = 4\varepsilon\left[\left(\frac{\sigma}{r}\right)^{12} - \left(\frac{\sigma}{r}\right)^{6}\right] + \varepsilon \qquad (1)$$

with a cutoff at $r = 2^{1/6}\sigma$.

The equations of motion for the particle positions $\mathbf{r}_i$ and orientation ($\theta$ in 2d and $\mathbf{p}_i$ in 3d) are:

$$\partial_t \mathbf{r}_i = \beta D_T\left[\mathbf{F}_i + F_p \mathbf{p}_i\right] + \sqrt{2D_T}\boldsymbol{\Lambda}_r\,, \qquad (2)$$

$$\partial_t \theta_i = \sqrt{2D_r}\Lambda_\theta\,, \quad (2d) \qquad (3)$$

$$\partial_t \mathbf{p}_i = \sqrt{2D_R}\left(\mathbf{p}_i \times \boldsymbol{\Lambda}_p\right)\,. \quad (3d) \qquad (4)$$

The translational and rotational diffusion constants $D_T$ and $D_R$ coupling is $D_T = D_R\sigma^2/3$. The inverse thermal energy scale is set to $\beta = 1/\varepsilon$. Following Stenhammar et al., we keep the self-propulsion force constant $F_p = 24\varepsilon/\sigma$ while varying the rotational diffusion constant and hence the Péclet number $\mathrm{Pe} = v_0/(\sigma D_r)$, where $v_0 = \beta D_t F_p$. The noise terms $\boldsymbol{\Lambda}_r, \boldsymbol{\Lambda}_\theta, \boldsymbol{\Lambda}_p$ are unit-variance stochastic vectors in three (or two) dimensions whose Cartesian components satisfy $\langle \Lambda_i(\mathbf{r},t)\Lambda_j(\mathbf{r}',t')\rangle = \delta_{ij}\delta(\mathbf{r}-\mathbf{r}')\delta(t-t')$. The rotational diffusion constant defines a natural timescale for the system, the rotational diffusion time $\tau_R = 1/D_R$.

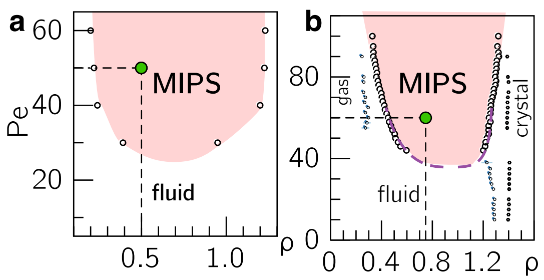


FIG. S1. MIPS phase diagrams for the (a) 2D and (b) 3D active Brownian particles. In our work we focus on state points well within the two phase region, running our simulations at Pe = 50, 60 in 2D/3D respectively. Green dots indicate the densities and Pe conditions of the simulations.

To integrate the equations of motion, we implement an Euler-Maruyama scheme with constant timestep $dt = 4\cdot 10^{-5}\tau_R$, following the Ermak–McCammon method described in detail in [2], with an in-house implementation for the molecular dynamics package LAMMPS [3].

In both 2d and 3d, ABPs exhibit motility induced phase separation between two disordered phases, a low density (gas-like) and a high density (liquid-like) phase, see Fig. S1. In 3d this separation is metastable with respect to gas-crystal phase separation.

In our simulations we perturb a uniform system by applying an external field. A static, local cosine barrier of potential $V_{\mathrm{ext}}(x) = \varepsilon_w\left[\cos(\pi x/d)+1\right]H(d-x)H(x+d)$ is imposed on the system and we attain steady state according to the following protocol:

- the $N$ particles are dispersed at random in the box;

* Corresponding author: f.turci@bristol.ac.uk

- 1000 steps of Fast Inertial Relaxation Engine (FIRE) minimisation removes any particle overlaps;

- the system is allowed to evolve for $1000\tau_R$ at constant Pe.

Typically we execute 10-40 independent runs, with further runs in cases where the system is less stable, principally at intermediate $\varepsilon_w$.

In two dimensions, we study systems at number density $\rho = 0.5$ with $L_x = 240\sigma$, and varying $L_y = 30, 60, 100, 120, 140, 160, 180\sigma$. This corresponds to particle numbers $N = 3600, 7200, 1200, 14\ 400, 16\ 800, 21\ 600$ respectively. In three dimensions we study systems at number density $\rho = 0.75$, with fixed $L_x = 100\sigma$ and varying $L_y = L_z = 16, 24, 32, 44\sigma$. This corresponds to particle numbers $N = 19\ 200, 43\ 200, 76\ 800, 145\ 200$. respectively

## S2. ASYMMETRY ORDER PARAMETER

In the main text we define the following order parameter to distinguish symmetric from asymmetric profiles

$$\mathcal{A}(t) = \left| \frac{\int_0^{L_x/2} \rho(x,t)dx - \int_{-L_x/2}^{0} \rho(x,t)dx}{(\rho - \rho_{\mathrm{LD}})L_x} \right|, \quad (5)$$

where $\rho(x,t)$ is the instantaneous density profile along the $x$-dimension (orthogonal to the barrier) and $L_x$ is the corresponding system size.

While the physical meaning of the numerator is self-evident, our choice for the normalisation constant at denominator is less obvious. Here we provide the rationale: We choose to work with a total density $\rho$ somewhat smaller than the diameter density $\bar{\rho} = (\rho_{\mathrm{LD}} + \rho_{\mathrm{HD}})/2$ between the MIPS coexisting densities $\rho_{\mathrm{LD}}, \rho_{\mathrm{HD}}$ so that less than half of the system is in the high density phase. A lever rule approximately holds for active Brownian particles, so that the fraction of the system in the high density phase is

$$f = \frac{\rho - \rho_{\mathrm{LD}}}{\rho_{\mathrm{HD}} - \rho_{\mathrm{LD}}}. \quad (6)$$

In the idealised case where the interfaces are sharp and the entire density profile is located in the positive semi-space (see Fig. S2), the numerator in equation 5 is

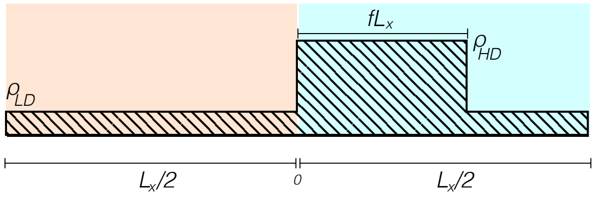


FIG. S2. Idealised asymmetric profile illustrating the definition of the order parameter, as described in the text.

$$\int_0^{L_x/2} \rho(x,t)dx - \int_{-L_x/2}^{0} \rho(x,t)dx = \quad (7)$$

$$= \rho_{\mathrm{HD}} f L_x + \rho_{\mathrm{LD}} \left( \frac{L_x}{2} - f L_x \right) - \rho_{\mathrm{LD}} \frac{L_x}{2} \quad (8)$$

$$= L_x \left( \rho_{\mathrm{HD}} f + \frac{\rho_{\mathrm{LD}}}{2} - \rho_{\mathrm{LD}} f - \frac{\rho_{\mathrm{LD}}}{2} \right) \quad (9)$$

$$= L_x \left( (\rho_{\mathrm{HD}} - \rho_{\mathrm{LD}}) f \right) = (\rho - \rho_{\mathrm{LD}}) L_x, \quad (10)$$

which serves to normalise the order parameter.

## S3. PHENOMENOLOGY OF WETTING TRANSITIONS IN SIMULATIONS WITH FIXED PARTICLE NUMBER

In equilibrium, the transition at constant temperature from complete to partial wetting can be explored for systems for which both the number of particles and the volume are fixed (the equilibrium NVT ensemble). For a fluid at liquid-gas coexistence and for sufficiently large $\rho$, these constraints generally lead to the formation of a slab of liquid which spans the systems via the periodic boundaries in $d-1$ dimensions. Early work [4] shows that for such a system confined in a slit-pore geometry by impenetrable walls that exert short-range attractive wall-fluid interactions, two possible states can occur as the strength of the attraction is varied:

1. *Complete wetting* in which the liquid slab splits in two and is adsorbed on both walls. This implies the formation of a *symmetric* density profile with four interfaces: wall-liquid, liquid-gas, gas-liquid and liquid-wall, see Fig. S3(a).

2. *Partial wetting*, where the wall-fluid attraction is insufficient to favour the formation of the liquid on both walls and the liquid slab is adsorbed on one of the two walls only. The state is therefore *asymmetric* and the system has only three interfaces: wall-liquid, liquid-gas, gas-wall, see Fig. S3(b).

This can be formalised using Young's equation

$$\gamma_{\mathrm{lg}}\cos\theta = \gamma_{\mathrm{wg}} - \gamma_{\mathrm{wl}} \tag{11}$$

In the complete wetting case, the total surface tension (free energy) from four interfaces is:

$$\gamma_{\mathrm{tot}} = 2\gamma_{\mathrm{wl}} + 2\gamma_{\mathrm{lg}}, \tag{12}$$

while in the partial wetting case the three interfaces give

$$\gamma_{\mathrm{tot}} = \gamma_{\mathrm{wl}} + \gamma_{\mathrm{lg}} + \gamma_{\mathrm{gw}}. \tag{13}$$

At the transition, $\cos\theta = 1$ and Eq. 11 yields $\gamma_{\mathrm{wg}} = \gamma_{\mathrm{lg}} + \gamma_{\mathrm{wl}}$. Plugging this into Eq. 13 we have that the total tension becomes $\gamma_{\mathrm{tot}} = \gamma_{\mathrm{wl}} + \gamma_{\mathrm{lg}} + \gamma_{\mathrm{lg}} + \gamma_{\mathrm{wl}} = 2\gamma_{\mathrm{wl}} + 2\gamma_{\mathrm{lg}}$ indicating that the asymmetric partial wetting state transforms into the symmetric one.

While in equilibrium there are various means of sampling the NVT ensemble (eg. a Langevin bath, deterministic thermostats or Monte-Carlo), our ABPs simulations Brownian dynamics with self-propulsion sample the NVPe ensemble which is closest in form to equilibrium simulations with Langevin or Brownian dynamics. The constraints of fixed N,V in our ABP simulation are sufficient to give rise to qualitatively equivalent behaviour in the coexistence region, namely liquid slab configurations.

In contrast to the equilibrium case where a purely repulsive impenetrable wall is always dry, in active systems it promotes complete wetting. We find that the propensity for wetting can be controlled by the magnitude of the repulsive strength of a finite energy barrier. When the repulsive strength is very high compared to the self-propulsion forces, the barrier is effectively impenetrable and we recover complete wetting. As in equilibrium, this state is *symmetric*, with the liquid adsorbed onto the barrier on both sides, see Fig. S3(c). As we decrease the barrier strength, however, the system spontaneously breaks the symmetry and, in analogy with the equilibrium case, an *asymmetric* density profile is formed, with a thicker region of liquid adsorbed only on one side of the barrier, see Fig. S3(d). Similarly to the equilibrium case, the two sides of the barrier are ultimately statistically equivalent, so inversion events can observed where the adsorbed liquid region shifts from one side to the other.

## S4. DETERMINATION OF BUBBLE SIZES

To extract the size of bubbles of the low density phase within the high density slab in contact with the external barrier we start from the discretisation of the instantaneous density field $\rho(\mathbf{r};t)$.

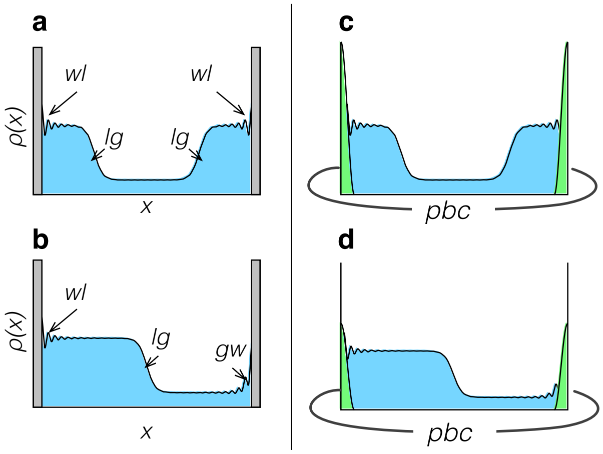


FIG. S3. Illustration of the relationship between profile symmetry and wetting/partial wetting. In (a-b) we give a schematic illustration of the equilibrium case in the presence of impenetrable walls with tuneable, short range attractions (grey rectangles) in a slit-pore geometry. (c-d) correspond to the active case, with a tuneable, finite-strength energy barrier (in green) in a system with periodic boundary conditions. In (a) and (b) we also indicate explicitly the interfaces that emerge: four interfaces for the symmetric case (a), three interfaces for the asymmetric case (b).

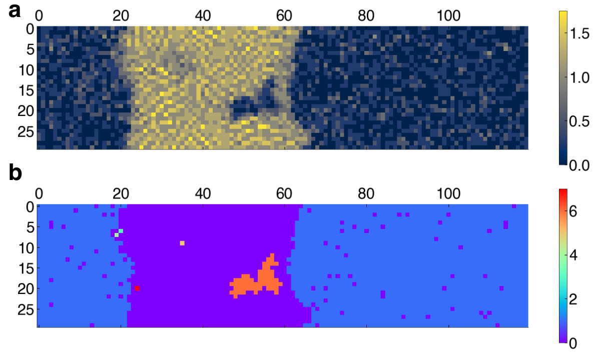


FIG. S4. Detection of bubbles in 2d: (a) the discretised density; (b) labelled connected regions, including a macroscopic bubble in the vicinity of the middle of the system close to the barrier which runs vertically at bin index 60. Values on the x-y axis indicate the bin index of the discretised profiles.

To illustrate the procedure, we consider the two-dimensional case. We produce two-dimensional histograms of $\rho(\mathbf{r};t)$ on grids of spacing $a = 2\sigma$. This produces a grayscale image of the density distribution which we threshold at $\rho_{\mathrm{mid}} = (\rho_{HD} + \rho_{LD})/2$ obtaining a binary image of low/high density regions. We then identify and label connected regions of low density, excluding those that span the peri-

odic boundaries.

To measure the size of such regions we retrieve the bounding box of each labelled region of low density and extract two lengths $\ell_{\parallel}, \ell_{\perp}$, parallel and orthogonal to the barrier respectively.

The statistics of bubble sizes is dominated by small bubbles, which are distributed all along the orthogonal dimension $x$. However, the relevant physical quantity is represented by the largest bubbles, which capture the growth of density fluctuations in the barrier region. In 2d the statistics for such extreme lengths depends on the barrier height, in particular in the parallel direction, see Fig.S5. For this reason, we characterise the tail of the probability distribution taking the average length of those whose length exceeds the 85th percentile of the population. We also tested other choices (90th and 95th percentiles) which do not affect the result significantly but (as they reduce the number of observations) increase the statistical error on the measured lengths.

## S5. SCALED COMPRESSIBILITY

The appearance of large bubbles is reflected in increased local density fluctuations. This can be quantified via a compressibility profile

$$\tilde{\chi}(x) = \left\langle (\delta N(x))^2 \right\rangle / \langle N(x) \rangle, \qquad (14)$$

where $N(x)$ is the lateral profile of number of particles.

Fig. S6(a) shows the behaviour of the scaled compressibility profile for the two-dimensional ABPs in a range of barrier strengths across the asymmetric-symmetric transition. The plot represents the profile so that the liquid is predominantly in the negative half-space. The profile exhibits large peaks corresponding to the fluctuations in the location of the liquid-vapor interfaces. A distinctive smaller peak at $x < 0$ close to $x = 0$ corresponds to enhanced bubble formation in the liquid phase near the barrier. Its height $\chi_0^{\max}$ provides a measure of the strength of density fluctuations around the barrier. In 2d, this height increases with decreasing barrier strength. In contrast, in three dimensions the fluctuations within the liquid display no significant dependence on the strength of the barrier, as shown in Fig. S6(b), indicating the absence of large correlation lengths.

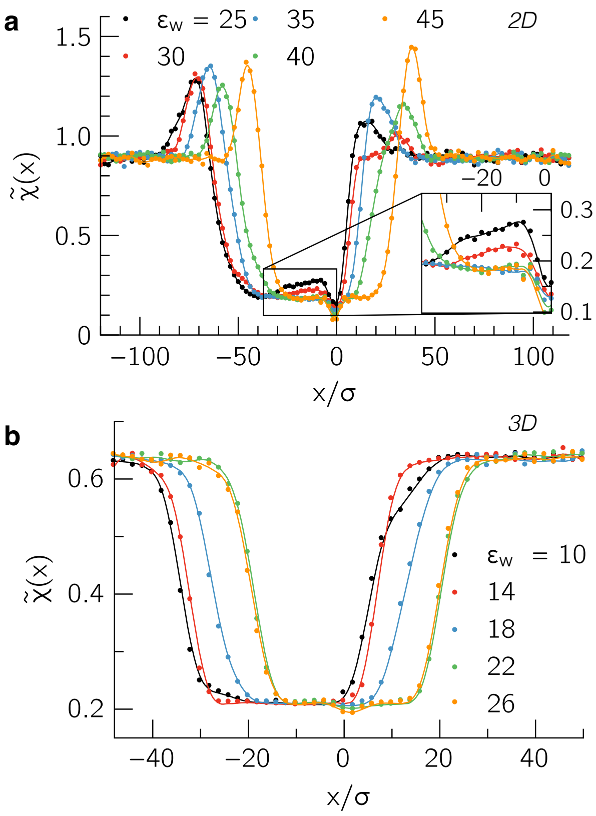


FIG. S6. (a) Measured form of the scaled compressibility profile for the two dimensional system for various values of the barrier strength. The zoomed inset shows the evolution of the peak contained within the liquid region in contact with the barrier. The system has size $L_x = 240\sigma, L_y = 120\sigma$ and $N = 14\ 400$. (b) Scaled compressibility profile for the three dimensional system across the asymmetric-to-symmetric transition. The liquid region at low compressibility presents no significant peaks with varying the barrier strength. The system has size $L_x = 100\sigma, L_y = L_z = 44\sigma$ and $N = 145\ 200$.

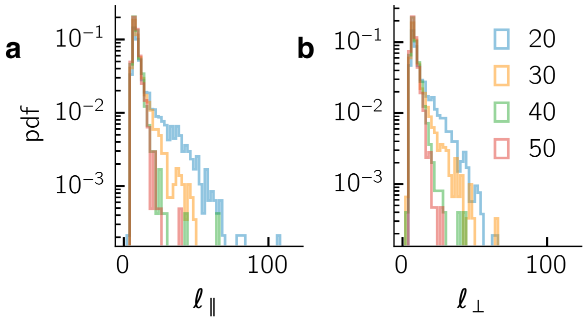


FIG. S5. Probability distributions of bubble sizes for the two-dimensional system for various values of the barrier strength $\varepsilon_{\mathrm{w}}$.

## S6. DETACHMENT FROM THE BARRIER

When the repulsive strength of the barrier $\varepsilon_w$ is sufficiently weak, the localisation of the high density phase becomes short-lived: the high density slabs detaches from the barrier and eventually diffuses away on the torus. Eventually, for zero $\varepsilon_w$, the steady state is simply the free diffusion of the slab on the torus due to periodic boundary conditions.

In 2d, detachment occurs because progressively larger bubbles of the low density phase are formed on the barrier as $\varepsilon_w$ is reduced. When the bubbles are as large as the transverse lengthscale $L_y$, the slab detaches. We can follow this process in space-time plots, see Fig. S7. We observe that while strong barriers lead to the formation of stable, symmetric density profiles which do not vary significantly over long timescales, weak barriers allow for the high density slab to cross, increase it asymmetry, fluctuate rapidly and eventually detach from the barrier at very late times. As shown in the figure, a thin layer of particles remains localised at the barrier even though the slab as a whole has detached.

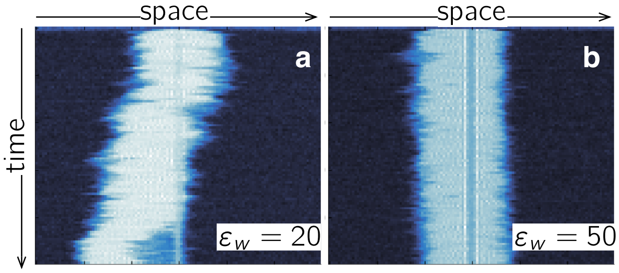


FIG. S7. Space-time plots of the density profiles in the two-dimensional system for (a) weak barrier, $\varepsilon_\mathrm{w} = 20$ and (b) strong barrier, $\varepsilon_\mathrm{w} = 50$. The timescale on both plots is $1000\tau_R$.

[1] J. Stenhammar, D. Marenduzzo, R. J. Allen, and M. Cates, Soft Matter **10**, 1489 (2014).
[2] S. Das, G. Gompper, and R. G. Winkler, New Journal of Physics **20**, 015001 (2018).
[3] S. Plimpton, Journal of Computational Physics **117**, 1 (1995).
[4] M. J. P. Nijmeijer, C. Bruin, A. F. Bakker, and J. M. J. van Leeuwen, Physical Review A **42**, 6052 (1990).
